# Supplementary material for: Parameterizing empirical interatomic potentials for predicting thermophysical properties via an irreducible derivative approach: the case of ThO$_2$ and UO$_2$
Source: arXiv:2204.13685 source file (2025-02-14)
Supplement: Supplementary file 1 [file table_sm_ids_of_2si.tex]

\begin{ruledtabular}
\begin{tabular}{@{}lcl}
\\[-1.0em]
$\CMcal{Q}$  & Count & Derivatives \\ [0.2em]
\hline\hline \\[-0.8em]
\multicolumn{3}{c}{Irreducible derivatives for $\CMcal{N}=2$, $ \mathbf{\hat{S}}_\mathrm{BZ}=2\mathbf{\hat{S}}_\mathrm{I}$ }\\[0.2em]
\colrule  \\[-0.8em]
$(\Gamma,\Gamma)$ & 2 & 
$d\indices*{*_{\Gamma}^{T_{2g}^{}}_{\Gamma}^{T_{2g}^{}}}$,
$d\indices*{*_{\Gamma}^{T_{1u}^{}}_{\Gamma}^{T_{1u}^{}}}$ \\ [0.4em]
$(X,X)$ & 7 & 
$d\indices*{*_{X}^{A_{1g}^{}}_{X}^{A_{1g}^{}}}$,
$d\indices*{*_{X}^{E_{g}^{}}_{X}^{E_{g}^{}}}$,
$d\indices*{*_{X}^{A_{2u}^{}}_{X}^{A_{2u}^{}}}$,
$d\indices*{*_{X}^{B_{1u}^{}}_{X}^{B_{1u}^{}}}$,
$d\indices*{*_{X}^{E_{u}^{}}_{X}^{E_{u}^{}}}$,
$d\indices*{*_{X}^{\tensor*[^{1}]{\hspace{-0.2em}E}{}_{u}^{}}_{X}^{\tensor*[^{1}]{\hspace{-0.2em}E}{}_{u}^{}}}$,
$d\indices*{*_{X}^{E_{u}^{}}_{X}^{\tensor*[^{1}]{\hspace{-0.2em}E}{}_{u}^{}}}$\\[0.8em]
\iffalse
$(L,L)$ & 8 & 
$d\indices*{*_{L}^{A_{1g}^{}}_{L}^{A_{1g}^{}}}$,
$d\indices*{*_{L}^{\tensor*[^{1}]{\hspace{-0.2em}A}{}_{1g}^{}}_{L}^{\tensor*[^{1}]{\hspace{-0.2em}A}{}_{1g}^{}}}$,
$d\indices*{*_{L}^{A_{1g}^{}}_{L}^{\tensor*[^{1}]{\hspace{-0.2em}A}{}_{1g}^{}}}$,
$d\indices*{*_{L}^{E_{g}^{}}_{L}^{E_{g}^{}}}$,
$d\indices*{*_{L}^{\tensor*[^{1}]{\hspace{-0.2em}E}{}_{g}^{}}_{L}^{\tensor*[^{1}]{\hspace{-0.2em}E}{}_{g}^{}}}$,
$d\indices*{*_{L}^{E_{g}^{}}_{L}^{\tensor*[^{1}]{\hspace{-0.2em}E}{}_{g}^{}}}$,
$d\indices*{*_{L}^{A_{2u}^{}}_{L}^{A_{2u}^{}}}$,
$d\indices*{*_{L}^{E_{u}^{}}_{L}^{E_{u}^{}}}$ \\[0.8em]
\fi
\multicolumn{3}{c}{Irreducible derivatives for $\CMcal{N}=3$, $ \mathbf{\hat{S}}_\mathrm{BZ}=2\mathbf{\hat{S}}_\mathrm{I}$ }\\[0.2em]
\colrule\\[-0.8em]
$(\Gamma,\Gamma,\Gamma)$ & 2 &  
$d\indices*{*_{\Gamma}^{T_{2g}^{}}_{\Gamma}^{T_{2g}^{}}_{\Gamma}^{T_{2g}^{}}}$,
$d\indices*{*_{\Gamma}^{T_{1u}^{}}_{\Gamma}^{T_{1u}^{}}_{\Gamma}^{T_{2g}^{}}}$ \\
\\[-0.8em]
$(\Gamma,X,X)$ & 17 & \makecell{ 
$d\indices*{*_{\Gamma}^{T_{2g}^{}}_{X}^{A_{1g}^{}}_{X}^{E_{g}^{}}}$, 
$d\indices*{*_{\Gamma}^{T_{2g}^{}}_{X}^{A_{2u}^{}}_{X}^{E_{u}^{}}}$,
$d\indices*{*_{\Gamma}^{T_{2g}^{}}_{X}^{A_{2u}^{}}_{X}^{\tensor*[^{1}]{\hspace{-0.2em}E}{}_{u}^{}}}$,  
$d\indices*{*_{\Gamma}^{T_{2g}^{}}_{X}^{B_{1u}^{}}_{X}^{E_{u}^{}}}$,
$d\indices*{*_{\Gamma}^{T_{2g}^{}}_{X}^{B_{1u}^{}}_{X}^{\tensor*[^{1}]{\hspace{-0.2em}E}{}_{u}^{}}}$,
$d\indices*{*_{\Gamma}^{T_{2g}^{}}_{X}^{E_{g}^{}}_{X}^{E_{g}^{}}}$, 
$d\indices*{*_{\Gamma}^{T_{2g}^{}}_{X}^{B_{1u}^{}}_{X}^{A_{2u}^{}}}$,
$d\indices*{*_{\Gamma}^{T_{2g}^{}}_{X}^{E_{u}^{}}_{X}^{E_{u}^{}}}$,\\ 
$d\indices*{*_{\Gamma}^{T_{2g}^{}}_{X}^{E_{u}^{}}_{X}^{\tensor*[^{1}]{\hspace{-0.2em}E}{}_{u}^{}}}$,  
$d\indices*{*_{\Gamma}^{T_{2g}^{}}_{X}^{\tensor*[^{1}]{\hspace{-0.2em}E}{}_{u}^{}}_{X}^{\tensor*[^{1}]{\hspace{-0.2em}E}{}_{u}^{}}}$,
$d\indices*{*_{\Gamma}^{T_{1u}^{}}_{X}^{A_{1g}^{}}_{X}^{E_{u}^{}}}$, 
$d\indices*{*_{\Gamma}^{T_{1u}^{}}_{X}^{A_{1g}^{}}_{X}^{\tensor*[^{1}]{\hspace{-0.2em}E}{}_{u}^{}}}$,   
$d\indices*{*_{\Gamma}^{T_{1u}^{}}_{X}^{B_{1u}^{}}_{X}^{E_{g}^{}}}$,
$d\indices*{*_{\Gamma}^{T_{1u}^{}}_{X}^{E_{g}^{}}_{X}^{A_{2u}^{}}}$, 
$d\indices*{*_{\Gamma}^{T_{1u}^{}}_{X}^{A_{1g}^{}}_{X}^{A_{2u}^{}}}$,
$d\indices*{*_{\Gamma}^{T_{1u}^{}}_{X}^{E_{g}^{}}_{X}^{E_{u}^{}}}$, \\  
$d\indices*{*_{\Gamma}^{T_{1u}^{}}_{X}^{E_{g}^{}}_{X}^{\tensor*[^{1}]{\hspace{-0.2em}E}{}_{u}^{}}}$,  
}\\
\\[-0.8em]
$(X,X,X)$ & 18 & \makecell{ 
$d\indices*{*_{X_{1}}^{A_{1g}^{}}_{X_{2}}^{A_{1g}^{}}_{X}^{A_{1g}^{}}}$, 
$d\indices*{*_{X_{1}}^{A_{1g}^{}}_{X_{2}}^{E_{g}^{}}_{X}^{E_{g}^{}}}$, 
$d\indices*{*_{X_{1}}^{A_{1g}^{}}_{X_{2}}^{A_{2u}^{}}_{X}^{E_{u}^{}}}$,
$d\indices*{*_{X_{1}}^{A_{1g}^{}}_{X_{2}}^{A_{2u}^{}}_{X}^{\tensor*[^{1}]{\hspace{-0.2em}E}{}_{u}^{}}}$,
$d\indices*{*_{X_{1}}^{A_{1g}^{}}_{X_{2}}^{B_{1u}^{}}_{X}^{B_{1u}^{}}}$, 
$d\indices*{*_{X_{1}}^{A_{1g}^{}}_{X_{2}}^{E_{u}^{}}_{X}^{E_{u}^{}}}$,   
$d\indices*{*_{X_{1}}^{A_{1g}^{}}_{X_{2}}^{E_{u}^{}}_{X}^{\tensor*[^{1}]{\hspace{-0.2em}E}{}_{u}^{}}}$,    
$d\indices*{*_{X_{1}}^{A_{1g}^{}}_{X_{2}}^{\tensor*[^{1}]{\hspace{-0.2em}E}{}_{u}^{}}_{X}^{\tensor*[^{1}]{\hspace{-0.2em}E}{}_{u}^{}}}$,\\
$d\indices*{*_{X_{1}}^{E_{g}^{}}_{X_{2}}^{E_{g}^{}}_{X}^{E_{g}^{}}}$,  
$d\indices*{*_{X_{1}}^{B_{1u}^{}}_{X_{2}}^{A_{2u}^{}}_{X}^{E_{g}^{}}}$,
$d\indices*{*_{X_{1}}^{B_{1u}^{}}_{X_{2}}^{E_{g}^{}}_{X}^{E_{u}^{}}}$, 
$d\indices*{*_{X_{1}}^{B_{1u}^{}}_{X_{2}}^{E_{g}^{}}_{X}^{\tensor*[^{1}]{\hspace{-0.2em}E}{}_{u}^{}}}$,     
$d\indices*{*_{X_{1}}^{E_{g}^{}}_{X_{2}}^{E_{u}^{}}_{X}^{A_{2u}^{}}}$,
$d\indices*{*_{X_{1}}^{E_{g}^{}}_{X_{2}}^{E_{u}^{}}_{X}^{E_{u}^{}}}$, 
$\tensor*[^{0}]{d}{}\indices*{*_{X_{1}}^{E_{g}^{}}_{X_{2}}^{E_{u}^{}}_{X}^{\tensor*[^{1}]{\hspace{-0.2em}E}{}_{u}^{}}}$,   
$d\indices*{*_{X_{1}}^{E_{g}^{}}_{X_{2}}^{\tensor*[^{1}]{\hspace{-0.2em}E}{}_{u}^{}}_{X}^{A_{2u}^{}}}$,       \\
$\tensor*[^{1}]{d}{}\indices*{*_{X_{1}}^{E_{g}^{}}_{X_{2}}^{E_{u}^{}}_{X}^{\tensor*[^{1}]{\hspace{-0.2em}E}{}_{u}^{}}}$,
$d\indices*{*_{X_{1}}^{E_{g}^{}}_{X_{2}}^{\tensor*[^{1}]{\hspace{-0.2em}E}{}_{u}^{}}_{X}^{\tensor*[^{1}]{\hspace{-0.2em}E}{}_{u}^{}}}$
}\\
\\[-0.8em]
\end{tabular}
\end{ruledtabular}
